# Supplementary material for: When Safe Models Merge into Danger: Exploiting Latent Vulnerabilities in LLM Fusion
Source: arXiv:2604.00627 source file (2026-04-01)
Supplement: Supplementary file 1 [file appendix.tex]

\begin{table}[ht]
\centering
\caption{Summary of key notations.}\vspace{-0.3cm}
\label{tab:notations}
\begin{tabularx}{\columnwidth}{lX}
\hline
\textbf{Symbol} & \textbf{Description} \\
\hline
\multicolumn{2}{l}{\textbf{General \& Model Merging Notations}} \\
$\mathcal{M}_i$, $\mathbf{M}^*$ & The $i$-th source model and the merged model. \\
$\theta_{\text{base}}$, $\theta_i$, $\theta_{\text{merged}}$ & Parameters of the base, a source, and the merged model. \\
$U, V$ & Up-projection and down-projection matrices in an MLP layer. \\
$\tau_i$ & Task vector for source model $\mathcal{M}_i$, defined as $\theta_i - \theta_{\text{base}}$. \\
\multicolumn{2}{l}{\textbf{Our Method (\name)}} \\
$X_{\text{malicious}}, X_s, X_u$ & Sets of malicious, safe, and unsafe input prompts. \\
$\Delta W$ & The target Safety-Critical Transformation (SCT) for the merged model. \\
$\Delta U_i$ & The latent attack component implanted into the matrix $U_i$. \\
$U'_i$ & The modified up-projection matrix after implanting the attack. \\
$\mathcal{L}_{1,i}$ & The \textbf{Source Safety} loss, ensuring alignment for malicious inputs. \\
$\mathcal{L}_{2,i}$ & The \textbf{Source Capacity} loss, preserving model functionality. \\
\hline
\end{tabularx}\vspace{-0.5cm}
\end{table}
